# Supplementary material for: HOPE: A Memory-Based and Composition-Aware Framework for Zero-Shot Learning with Hopfield Network and Soft Mixture of Experts
Source: arXiv:2311.14747 source file (2025-03-10)
Supplement: Supplementary file 1 [file appendix.tex]

\section{Impact of Hyperparameter on Accuracy \& Convergence:}
Figure \ref{hyperparams} shows that despite using different hyperparameter configurations, the accuracy on both unseen and seen data consistently converges to a similar value. The primary difference is in the speed of this convergence, with a slight performance drop observed when $\alpha$ and $\beta$ are significantly larger than $\gamma$.
\begin{figure*}[!ht]
    \vspace{-1em}
    \centering
    \includegraphics[width=0.9\textwidth]{images/combined_accuracy_plot.png}
    \caption{Seen (S) and Unseen (U) accuracy in different set of ($\alpha, \beta, \gamma$)}
    \label{hyperparams}
    \vspace{-1.5em}
\end{figure*}
\clearpage
\section{Evaluations}
We provide experimental comparisons in Tables~\ref{closed-world} and \ref{open-world} against all previously established compositional zero-shot learning methods, including AoP \cite{nagarajan2018attributes}, LE+ \cite{naeem2021learning}, TMN \cite{purushwalkam2019task}, SymNet \cite{li2020symmetry}, CompCos \cite{mancini2021open}, CGE \cite{naeem2021learning}, Co-CGE \cite{mancini2022learning}, SCEN \cite{li2022siamese}, KG-SP \cite{karthik2022kg}, CSP \cite{nayak2022learning}, and DFSP \cite{lu2023decomposed}. Performance is assessed in both closed-world and open-world scenarios.
\begin{table*}[!htb]
    \begin{center}
    \fontsize{9}{11}\selectfont
        \begin{tabular}{c|c c c c | c c c c | c c c c|}
             \multirow{2}{5em}{Method} &  \multicolumn{4}{|c|}{MIT-States} & \multicolumn{4}{|c|}{UT-Zappos} & \multicolumn{4}{|c|} {C-GQA}\\
             & S & U &  H & AUC & S & U &  H & AUC & S & U &  H & AUC \\
             \hline
             AoP \cite{nagarajan2018attributes} & 14.3 & 17.4 & 9.9 & 1.6 & 59.8 & 54.2 & 40.8 & 25.9 & 17.0 & 5.6 & 5.9 & 0.7 \\
             LE+ \cite{naeem2021learning} & 15.0 & 20.1 & 10.7 & 2.0 & 53.0 & 61.9 & 41.0 & 25.7 & 18.1 & 5.6 & 6.1 & 0.8 \\
             TMN \cite{purushwalkam2019task} & 20.2 & 20.1 & 13.0 & 2.9 & 58.7 & 60.0 & 45.0 & 29.3 & 23.1 & 6.5 & 7.5 & 1.1 \\
             SymNet \cite{li2020symmetry} & 24.2 & 25.2 & 16.1 & 3.0 & 49.8 & 57.4 & 40.4 & 23.4 & 26.8 & 10.3 & 11.0 & 2.1 \\
             CompCos \cite{mancini2021open} & 25.3 & 24.6 & 16.4 & 4.5 & 59.8 & 62.5 & 43.1 & 28.1 & 28.1 & 11.2 & 12.4 & 2.6 \\
             CGE \cite{naeem2021learning} & 31.1 & 5.8 & 6.4 & 1.1 & 62.0 & 44.3 & 40.3 & 23.1 & 32.1 & 2.0 & 3.4 & 0.5 \\
             Co-CGE \cite{mancini2022learning} &  31.1 & 5.8 & 6.4 & 1.1 & 62.0 & 44.3 & 40.3 & 23.1 & 32.1 & 2.0 & 3.4 & 0.5 \\
             SCEN \cite{li2022siamese} & 29.9 & 25.2 & 18.4 & 5.3 & 63.5 & 63.1 & 47.8 & 32.0 & 28.9 & 25.4 & 17.5 & 5.5\\
             CLIP \cite{radford2021learning} & 30.2 & 45.9 & 26.1 & 11.1 & 15.8 & 49.2 & 15.6 & 5.0 & 7.7 & 24.8 & 8.4 & 1.3 \\
             CSP \cite{nayak2022learning} & 46.6 & 49.9 & 36.3 & 19.4 & 64.2 & 66.2 & 46.6 & 33.0 & 28.8 & 26.8 & 20.5 & 6.2  \\
             CSP \cite{nayak2022learning} & 46.6 & 49.9 & 36.3 & 19.4 & 64.2 & 66.2 & 46.6 & 33.0 & 28.8 & 26.8 & 20.5 & 6.2  \\
             DFSP \cite{lu2023decomposed} & 46.9 & 52.0 & 37.3 & 20.6 & 66.7 & 71.7 & 47.2 & 36.0 & \textbf{38.2} & \textbf{32.0} & \textbf{27.1} & \textbf{10.5}\\
             \hline
            \textbf{HOMOE} & \textbf{50.5} & \textbf{54.6} & \textbf{39.9} & \textbf{23.3} & \textbf{68.4} & \textbf{73.9} & \textbf{49.1} & \textbf{37.5} & 35.8 & 30.8 & 24.5 & 9.1\\
             \hline
        \end{tabular}
        \caption{\label{closed-world} Closed World Evaluation. Comparison to state-of-the-art models}
    \end{center}
\vspace{-.5cm}
\end{table*}

\begin{table*}[!htb]
    \begin{center}
    \fontsize{9}{11}\selectfont
        \begin{tabular}{c|c c c c | c c c c | c c c c|}
             \multirow{2}{5em}{Method} &  \multicolumn{4}{|c|}{MIT-States} & \multicolumn{4}{|c|}{UT-Zappos} & \multicolumn{4}{|c|}{C-GQA}\\
             & S & U &  H & AUC & S & U &  H & AUC & S & U &  H & AUC \\
             \hline
             AoP \cite{nagarajan2018attributes} & 16.6 & 5.7 & 4.7 & 0.7 & 50.9 & 34.2 & 29.4 & 13.7 & - & - & - & - \\
             LE+ \cite{naeem2021learning} & 14.2 & 2.5 & 2.7 & 0.3 & 60.4 & 36.5 & 30.5 & 16.3 & 19.2 & 0.7 & 1.0 & 0.08 \\
             TMN \cite{nayak2022learning} & 12.6 & 0.9 & 1.2 & 0.1 & 55.9 & 18.1 & 21.7 & 8.4 & - & - & - & - \\
             SymNet \cite{li2020symmetry} & 21.4 & 7.0 & 5.8 & 0.8 & 53.3 & 44.6 & 34.5 & 18.5 & 26.7 & 2.2 & 3.3 & 0.43 \\
             CompCos \cite{mancini2021open} & 25.4 & 10.0 & 8.9 & 1.6 & 59.3 & 46.8 & 36.9 & 21.3 & - & - & - & - \\
             CGE \cite{naeem2021learning} & 32.4 & 5.1 & 6.0 & 1.0 & 61.7 & 47.7 & 39.0 & 23.1 & 32.7 & 1.8 & 2.9 & 0.47 \\
             Co-CGEˆClosed \cite{mancini2022learning} & 31.1 & 5.8 & 6.4 & 1.1 & 62.0 & 44.3 & 40.3 & 23.1 & 32.1 & 2.0 & 3.4 & 0.53 \\
             Co-CGEˆOpen \cite{mancini2022learning} & 30.3 & 11.2 & 10.7 & 2.3 & 61.2 & 45.8 & 40.8 & 23.3 & 32.1 & 3.0 & 4.8 & 0.78 \\
             KG-SP \cite{karthik2022kg} & 28.4 & 7.5 & 7.4 & 1.3 & 61.8 & 52.1 & 42.3 & 26.5 & 31.5 & 2.9 & 4.7 & 0.78 \\
             DRANet \cite{li2023distilled} & 29.8 & 7.8 & 7.9 & 1.5 & 65.1 & 54.3 & 44.0 & 28.8 & 31.3 & 3.9 & 6.0 & 1.05 \\ 
            CLIP \cite{radford2021learning} & 30.1 & 14.3 & 12.8 & 3.0 & 15.6 & 20.5 & 11.3 & 2.2 & 7.5 & 4.4 & 4.0 & 0.28 \\
             CSP \cite{nayak2022learning} & 46.3 & 15.7 & 17.4 & 5.7& 64.1 & 44.1 & 38.9 & 22.7 & 28.7 & 5.2 & 6.9 & 1.2  \\
             DFSP \cite{lu2023decomposed} & 47.5 & 18.5 & 19.3 & 5.8 & 66.8 & 60.0 & 44.0 & 30.3 & \textbf{38.3} & \textbf{7.2} & \textbf{10.4} & \textbf{2.4}\\
             \hline
            \textbf{HOMOE} & \textbf{50.4} & \textbf{19.7} & \textbf{20.7} & \textbf{7.9} & \textbf{68.4} & \textbf{61.9} & \textbf{45.1} & \textbf{31.1} & 35.7 & 6.6 & 9.0 & 2.0\\
             \hline
        \end{tabular}
        \caption{\label{open-world} Open World Evaluation. Comparison to state-of-the-art models}
    \end{center}
\vspace{-.7cm}
\end{table*}
